# Supplementary material for: ArchesWeather: An efficient AI weather forecasting model at 1.5{\deg} resolution
Source: arXiv:2405.14527 source file (2024-07-03)
Supplement: Supplementary file 1 [file appendix.tex]

\section{Training cost calculations}

We consider 
1 A100 = 2 V100,
1 TPUv4 = 3 V100,
1 TPUv5e = 6 V100

\section{Comparison to state of the art}
Spherical CNN is trained every 3hours, compared to 6h for Stormer and for our model

Stormer was evaluated at 1.4º resolution with model outputs provided by the authors
